# Supplementary material for: ArtiFix: Localizing and Repairing Artifacts in AI-Generated Videos
Source: arXiv:2611.40165 source file (2026-11-29)
Supplement: Supplementary file 1 [file fig_pipeline_supp.tex]

% Graphic in figures/assets/, generated by artifact_pipeline/scripts/fig_pipeline_split.py (supplementary panel).
\begin{figure*}[t]
\centering
\includegraphics[width=\textwidth]{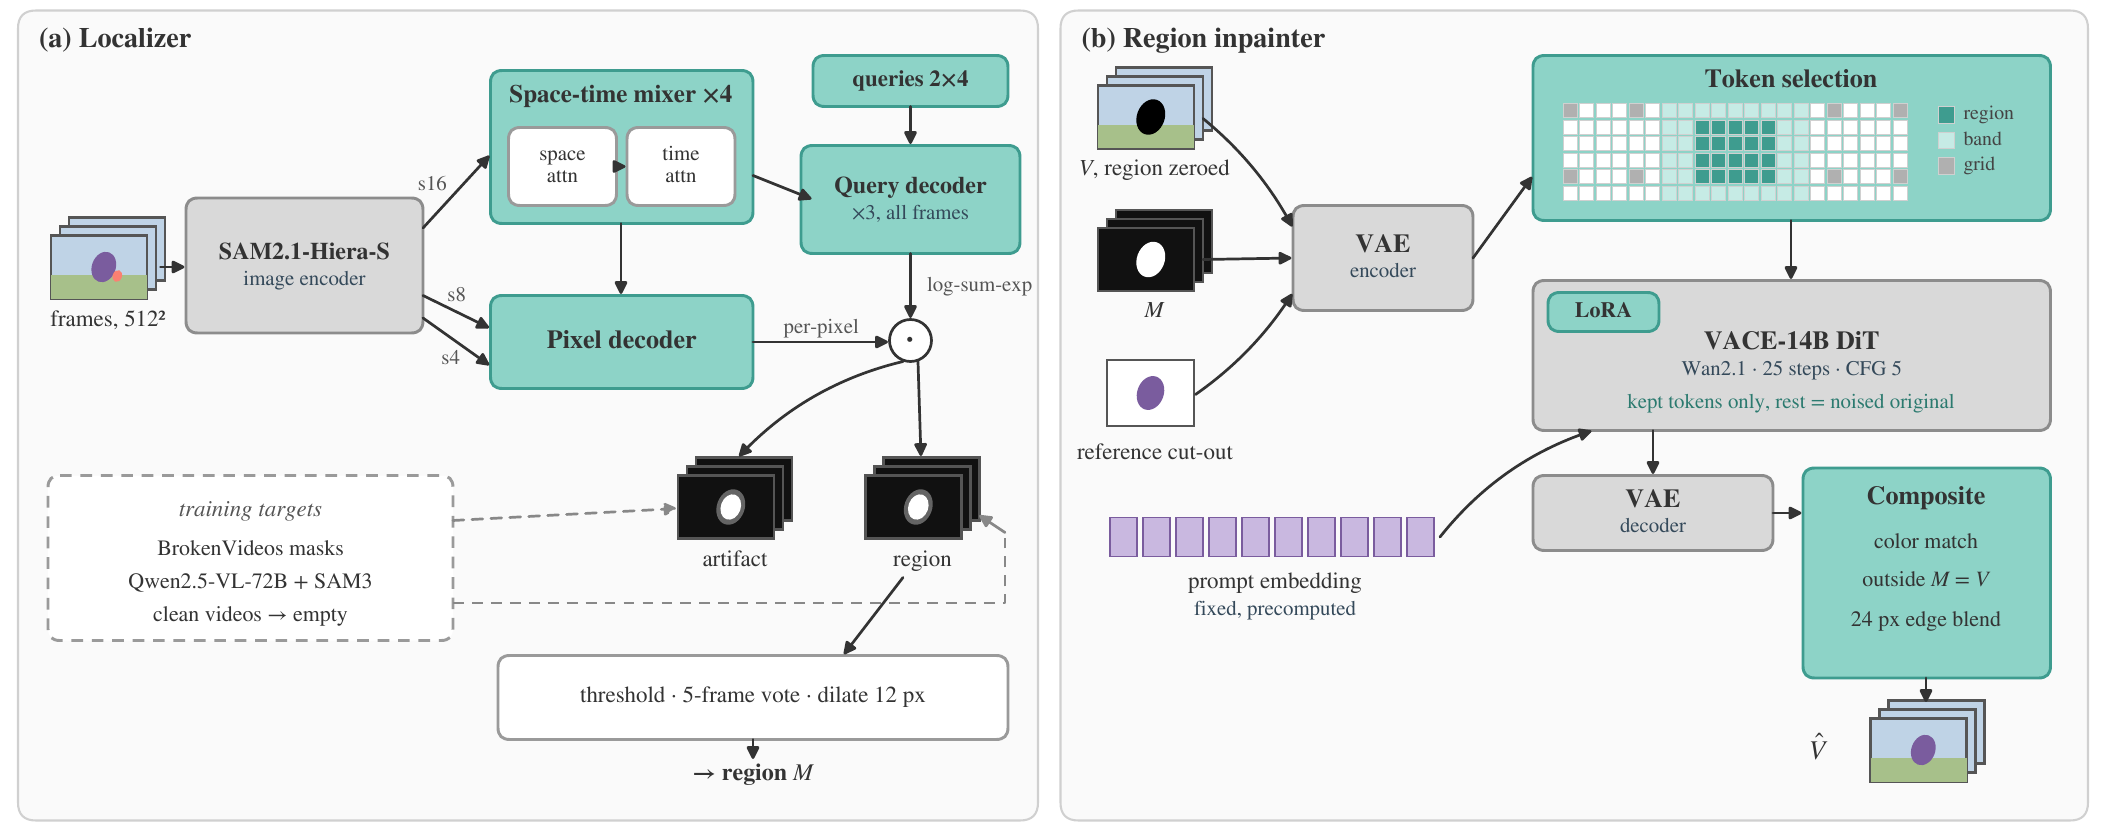}
\caption{Layers of the pipeline. (a) The localizer encodes frames with a frozen SAM2.1 encoder, mixes them over space
and time, and decodes an artifact map and a region map with learned queries. (b) The inpainter encodes the video with
the region set to zero, the mask and a reference cut-out of the object, uses a fixed prompt embedding, and runs
VACE-14B with the LoRA only on the region, a band around it and a sparse grid of tokens before the composite.}
\label{fig:supp_pipeline}
\end{figure*}
