# Supplementary material for: ArtiFix: Localizing and Repairing Artifacts in AI-Generated Videos
Source: arXiv:2611.40165 source file (2026-11-29)
Supplement: Supplementary file 2 [file supp_block_fn.tex]

% Negative (where our region misses part of the annotated artifact), added on the owner's request (11-22).
% Self-contained, comment out its \input line to drop it. Graphic: artifact_pipeline/scripts/fig_supp_visuals.py fn
On 7 of the 103 test clips our region covers less than 80\% of the annotated artifact pixels, and \cref{fig:supp_fn} shows the four with the lowest coverage, where the region leaves out part of what the annotation marks.\TODO{Negative result, review: partial misses of the localizer.}

\begin{figure}[t]
\centering
\includegraphics[width=\linewidth]{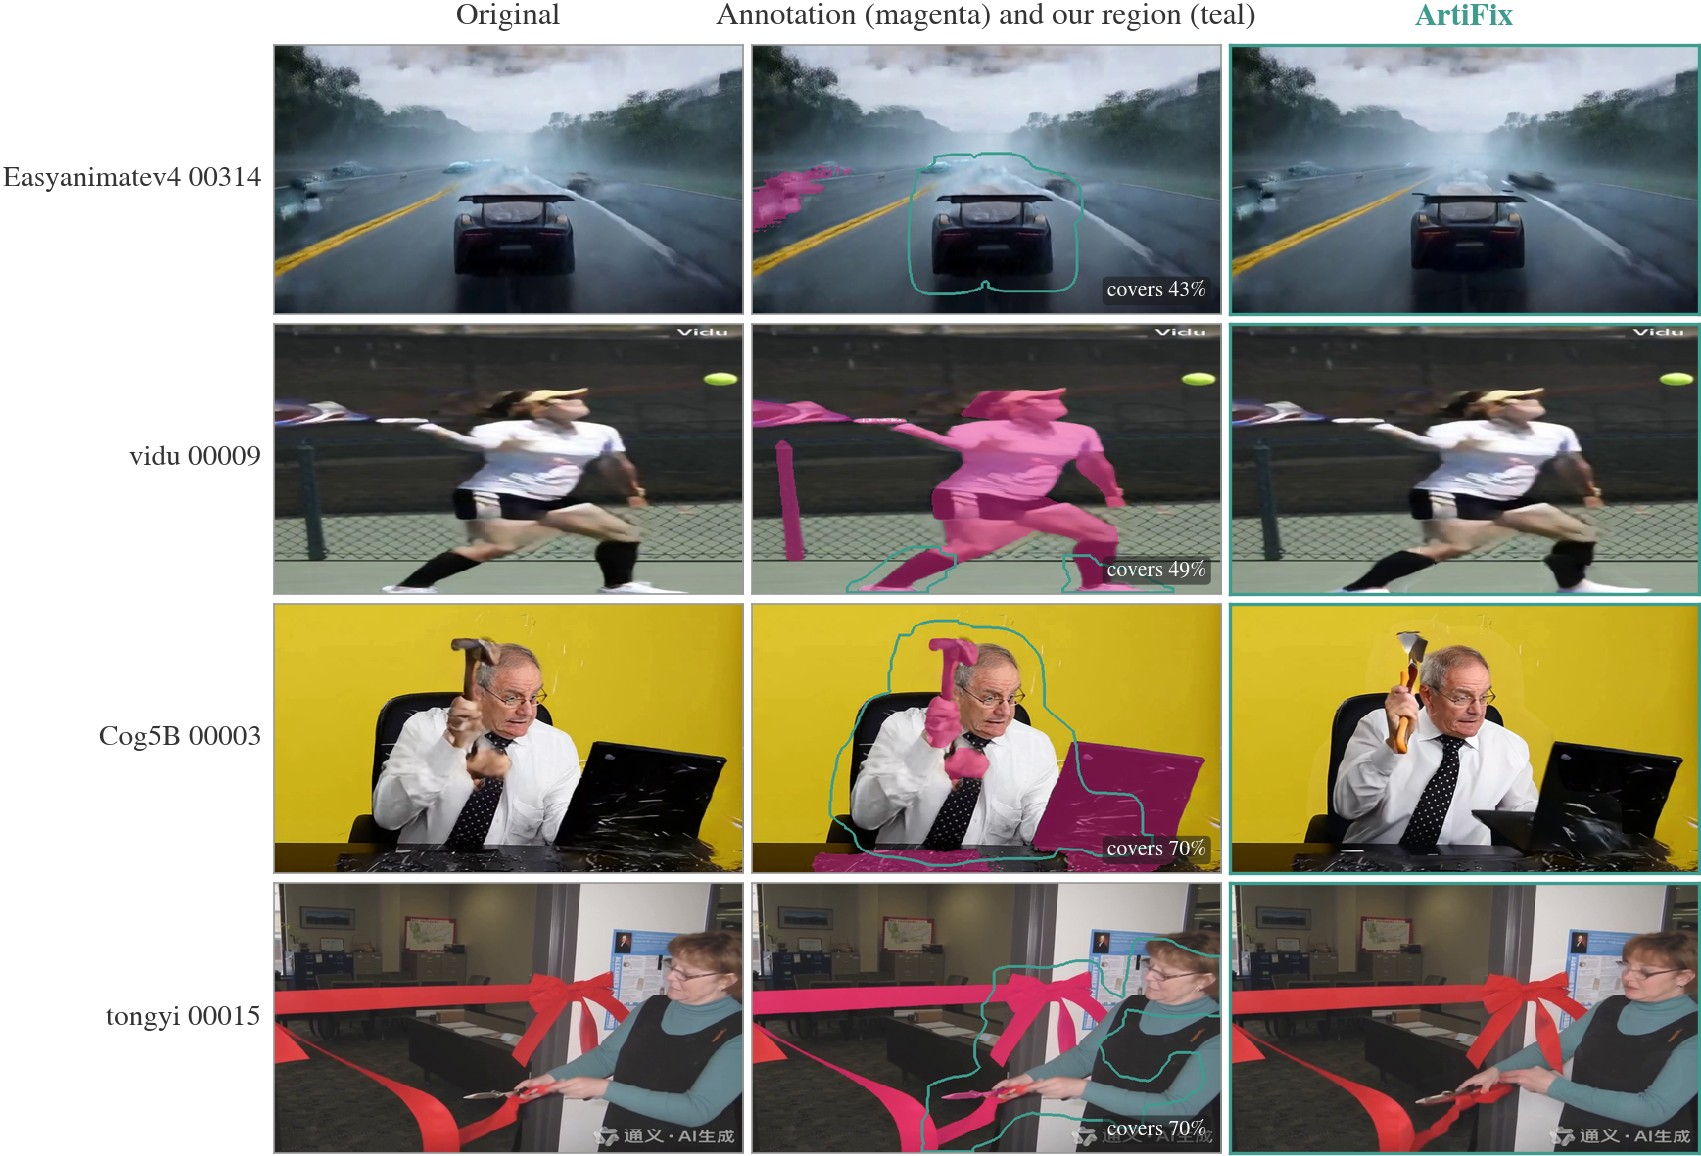}
%\caption{The four test clips where our region covers the least of the annotated artifact, at the frame where the most annotated pixels fall outside it. The share of annotated pixels covered by our region is given on each.}
\caption{\textbf{Where our region misses part of the artifact.} The four test clips where our region covers the least of the annotated artifact, at the frame where the most annotated pixels fall outside it. The share of annotated pixels covered by our region is given on each.}
\label{fig:supp_fn}
\end{figure}
